# Supplementary material for: Microlayer in nucleate boiling seen as Landau-Levich film with dewetting and evaporation
Source: arXiv:2306.09838 source file (2023-06-16)
Supplement: Supplementary file 1 [file SupportingInfo1.pdf]

# Supporting information for "Microlayer in nucleate boiling seen as Landau-Levich film with dewetting and evaporation"

Cassiano Tecchio,[1] Xiaolong Zhang (张晓龙),[2] Benjamin Cariteau,[1] Gilbert Zalczer,[2] Pere Roca i Cabarrocas,[3] Pavel Bulkin,[3] Jérôme Charliac,[3] Simon Vassant,[2] and Vadim S. Nikolayev[2]

[1]*STMF, CEA, Université Paris-Saclay, 91191 Gif-sur-Yvette Cedex, France*

[2]*SPEC, CEA, CNRS, Université Paris-Saclay, 91191 Gif-sur-Yvette Cedex, France*

[3]*LPICM, CNRS, Ecole Polytechnique, Institut Polytechnique de Paris, 91120 Palaiseau, France*

(*cassiano.tecchio@cea.fr)

(Dated: June 16, 2023)

## I. WHITE LIGHT INTERFEROMETRY

### A. Calibration

The aim of calibration is to relate the pixel sequential numbers ($x'$ and $\lambda'$) along the axes to $x$ and $\lambda$, both in meters, respectively.

- Ordinate axis: By using the $MgF_2$ porthole without ITO (to avoid interference) an optical color filter (corresponding to the wavelength $\lambda$) is placed between the light source and the visible light beam splitter which results in a horizontal bright stripe at $\lambda'$. Ten different filters are used, one at a time. Figure 1a shows the relationship

$$\lambda = a(\lambda' - 1) + \lambda_{min}, \qquad (1)$$

where the slope $a = 0.1624\,\mathrm{nm/px}$ represents the spectral resolution of our optical system. $\lambda_{min} = 437.24\,\mathrm{nm}$ is the lowest visible wavelength. $\lambda'$ ranges from 1 to 1280 px, which is the camera matrix vertical size. The visible spectrum bandwidth is then $\lambda_{min} \leq \lambda \leq \lambda_{max}$, where $\lambda_{max} = 644.95\,\mathrm{nm}$. The uncertainties on $a$ and on $\lambda$ are $\pm 0.002\,\mathrm{nm/px}$ and $\pm 2.5\,\mathrm{nm}$, respectively, for the confidence level of 95%.

- Abscissa axis is calibrated by imaging the square optical target with known dimensions printed on it. The spectrometer is used in mirror mode. Fig. 1b shows the calibration curve.

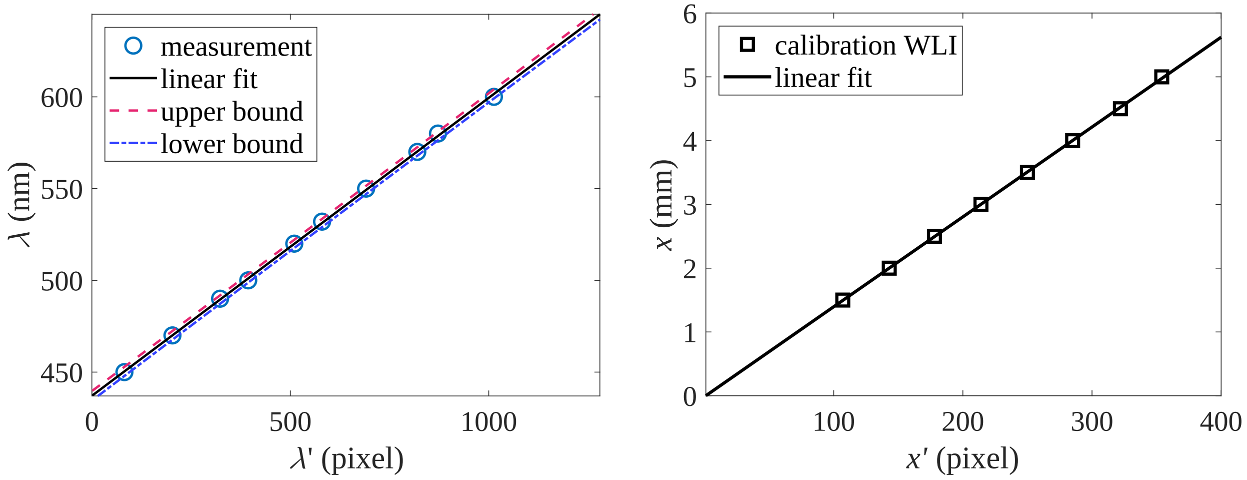


(a) Relationship between camera vertical axis $\lambda'$ and wavelength $\lambda$.

(b) Relationship between camera horizontal axis $x'$ and $x$ along the scanning line.

FIG. 1. Calibration in white light interferometry.

$x$ and $x'$ are given in meters and pixels, respectively. The horizontal axis follows a relation in the form of

$$x = \mathsf{K}x', \tag{2}$$

where $\mathsf{K} = 14.09\,\mu\mathrm{m/px}$, i.e., a horizontal pixel size corresponds to 14.09 µm along the heater. The linearity confirms the absence of optical distortions. The uncertainty of $x$ can then be taken as one pixel size.

### B. Data reduction

To obtain the microlayer thickness from the spectral fringe map, we use the methodology proposed by Glovnea *et al.* [1] where the function $F$, defined as

$$F = \sum_{\lambda_{min} \le \lambda \le \lambda_{max}} \left[I_{c,exp}(\lambda) - \mathscr{K} I_{theo}(\lambda)\right]^2, \tag{3}$$

is minimized. $I_{c,exp}(\lambda)$ and $I_{theo}(\lambda)$ represent the experimental and theoretical intensity distributions along $\lambda$ for a fixed $r$. The experimental intensity $I_{c,exp}(\lambda) = I_{exp}(\lambda)/I_s(\lambda)$ is compensated to eliminate the effect of uneven spectral intensity emission from the light source. $I_{exp}$ is the uncompensated camera output and $I_s(\lambda)$ is obtained from a preliminary experiment at equilibrium with the bare $MgF_2$ porthole (without the ITO). $\mathscr{K}$ is a scaling factor that accounts for the different intensity span in the measurements.

The theoretical distribution $I_{theo}(\lambda)$ is obtained by modeling the intensity of the light that is reflected from the interfaces determined by the $MgF_2$, ITO, microlayer and vapor. The transmittance (through the $MgF_2$, ITO and microlayer) and the absorbance by the ITO are taken into account by Fresnel equations and a fitting parameter that accounts for the actual light dispersion during the experiment, respectively [2].

The $F$ minimization is first performed for each point along $r$ axis to get ITO film using $I_{c,exp}(\lambda)$ obtained prior to the bubble nucleation and $I_{theo}(\lambda)$ that corresponds to the interference on the ITO film only; its local thickness can be calculated with precision at this step. In the second step, $\delta$ is determined with a similar minimization procedure but using the time-dependent fringe pattern $I_{c,exp}(\lambda)$ obtained during the bubble growth (right middle image in Fig. 1 of the main article) where $I_{theo}(\lambda)$ corresponds to the interference on both the ITO film and the microlayer; is thus a function of already known ITO thickness and $\delta$. For each $x$, the $F$ minimization gives the $\delta$ value as the best fit.

The image processing was validated by using the plano-convex lens with the radius of curvature $\mathtt{R}$ given by the manufacturer. The lens was posed on the porthole with a convex side downward thus forming an air layer of the thickness $\delta(r)$. Its theoretical value could thus be determined from the equation

$$(\mathtt{R}-\delta)^2+r^2-\mathtt{R}^2=0, \tag{4}$$

where $r$ was the horizontal coordinate axis on the porthole centered at the point of symmetry of the lens. The experimental data agreed with this theoretical value within 40 nm between 0.1 and 6 $\mu$m (which is a much better agreement than that of Jung and Kim [3].

## II. IR THERMOGRAPHY

Prior to the boiling experiment, the temperature of the boiling cell is raised up to 100 °C by reaching stationary conditions where the cell can be considered at thermal equilibrium. The preliminarily calibrated RTD is placed close to the ITO surface so that the RTD measurement gives the wall (i.e. ITO film) temperature $T_w$. It can be related to the intensity $I$ of the IR radiation emitted by the ITO and captured by the IR camera. The theoretical expression of $I(T_w)$ is

$$I(T_w)=\int_{\lambda_1}^{\lambda_2}\mathscr{R}_{hm}(\lambda)\mathscr{S}_{IR,det}(\lambda)\mathscr{T}_{IR,obj}(\lambda)W^b(\lambda,T_w)d\lambda; \tag{5}$$

where

$$W^b(\lambda, T_w) = \frac{C_1}{\lambda^5 \left[\exp(\frac{C_2}{\lambda T_w}) - 1\right]}; \tag{6}$$

is the Plank law. $C_1 = 3.74 \times 10^{-16}\,\mathrm{W\,m^2}$ and $C_2 = 1.44 \times 10^{-2}\,\mathrm{m\,K}$ represent the first and second radiation constants. The integration is performed within the camera bandwidth, $\lambda_1 = 2.5\,\mu\mathrm{m}$ and $\lambda_2 = 5.5\,\mu\mathrm{m}$. $\mathscr{S}_{IR,det}(\lambda)$ and $\mathscr{T}_{obj}(\lambda)$ represent the sensitivity of the IR detector and the transmittance of the objective, respectively. They were obtained from the camera manufacturer. $\mathscr{R}_{hm}(\lambda)$ is the reflectance of the visible-IR light beam splitter. It has been measured [2] by FTIR (Fourier-Transform Infrared Spectroscopy).

One is interested in the function $T_w = T_w(I)$ inverse to $I(T_w)$. Schweikert *et al.* [4] proposed the fit

$$T_w = A_1 \left[(I + A_2)^{1/4} + A_3\right]; \tag{7}$$

where $A_1$, $A_2$ and $A_3$ are constants that account for the surrounding radiation, ITO emissivity and attenuation in the atmosphere. The calibration is pixel-wise. This means that each pixel has its own fitting coefficients, which avoids errors due to vignetting. Figure 2a shows that Eq. (7) indeed fits the theoretical law (5) for a wide range of $T_w$ with a small error of $0.07\,^\circ\mathrm{C}$. Therefore, one can use Eq. (7) for calibration.

Figure 2b shows an example of calibration for a given pixel. Six calibration points are obtained within the range $50\,^\circ\mathrm{C} \le T_w \le 100\,^\circ\mathrm{C}$. Equation (7) is used for fitting. The root mean square fitting error is 0.4 K. The cell is at atmospheric pressure, so calibration beyond the saturation temperature is impossible. During the bubble growth, $T_w > T_{sat}$ and we need to extrapolate the fit. However, the error is expected to be minor thanks to the use of a physically justified fit; the uncertainty of $T_w$ is estimated to be $\pm 0.5\,\mathrm{K}$.

The spatial resolution for the IR thermography has been calibrated by imaging the hole of a known diameter. It is $84\,\mu\mathrm{m/px}$ along both the horizontal and vertical axes of the IR camera image.

---


[1] R. Glovnea, A. Forrest, A. Olver, and H. Spikes, Measurement of sub-nanometer lubricant films using ultra-thin film interferometry, Tribol. Lett. **15**, 217 (2003).

[2] C. Tecchio, *Experimental study of boiling: characterization of near-wall phenomena and bubble dynamics*, Ph.D. thesis, Paris-Saclay University (2022).

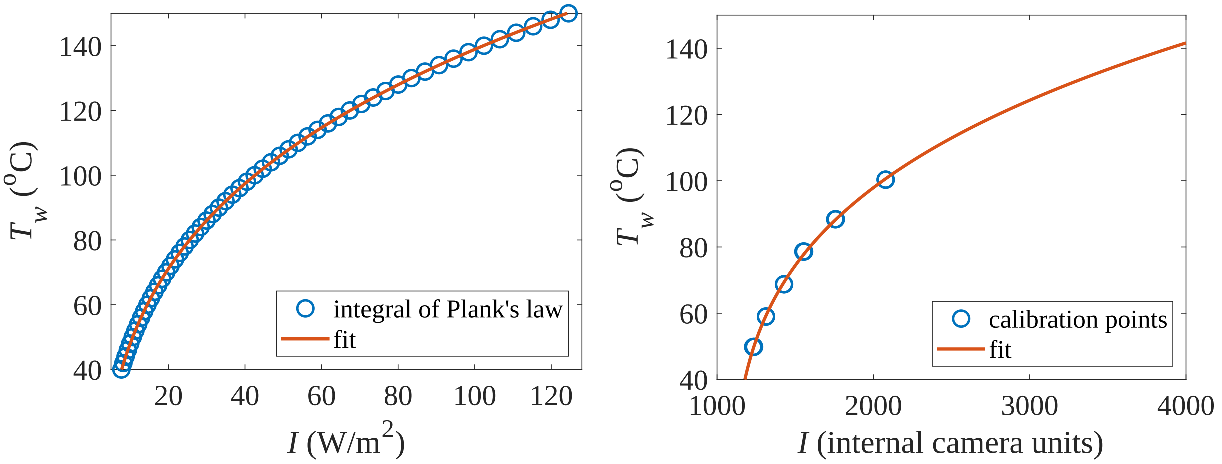


(a) Fit (7) of the theoretical Eq. (5).

(b) An example of the fit (7) of the signal from a camera pixel.

FIG. 2. IR thermography calibration.

[3] S. Jung and H. Kim, Hydrodynamic formation of a microlayer underneath a boiling bubble, Int. J. Heat Mass Transf. **120**, 1229 (2018).

[4] K. Schweikert, A. Sielaff, and P. Stephan, Pixel-wise in situ calibration method for high accuracy infrared thermography of moving targets, Infrared Phys. Technol. **118**, 103862 (2021).
